# Supplementary material for: From Following to Understanding: Investigating the Role of Reflective Prompts in AR-Guided Tasks to Promote Task Understanding
Source: arXiv:2501.13258 source file (2025-01-22)
Supplement: Supplementary file 1 [file 8-appendix.tex]

% \appendix
% \section{Quizzes for Objective Understanding Assessment}\label{app:quizzes}
% Below is the quiz for Task A.
% \begin{enumerate}[label=\textbf{Q\arabic*.}]
%     \item What is the typical coffee-to-water ratio range for pour-over brewing?
%     \begin{tasks}(2)
%         \task 1:10 to 1:12
%         \task 1:15 to 1:17
%         \task 1:20 to 1:22
%         \task 1:25 to 1:27
%     \end{tasks}

%     \item What type of coffee bean did we use?
%     \begin{tasks}(2)  % 1 column
%         \task Light roast
%         \task Medium roast
%         \task Medium-dark roast
%         \task Dark roast
%     \end{tasks}

%     \item After adding ground coffee to the filter, what is the next step in the pour-over process?
%     \begin{tasks}(2)
%         \task Start the main pour
%         \task Bloom the coffee
%         \task Stir the grounds
%         \task Tap the filter to settle the grounds
%     \end{tasks}

%     \item How much water do you typically need for the blooming step?
%     \begin{tasks}(2)
%         \task About half the total brewing water
%         \task Just enough to wet all the grounds
%         \task Approximately twice the weight of the coffee
%         \task One-third of the total brewing water
%     \end{tasks}

%     \item What problem might occur if you don't pre-wet the paper filter?
%     \begin{tasks}(2)
%         \task The coffee will be too strong
%         \task The filter might collapse
%         \task The coffee may have a papery taste
%         \task The extraction will be too fast
%     \end{tasks}

%     \item Which pouring technique is recommended for achieving even extraction after the bloom phase?
%     \begin{tasks}(2)
%         \task Pour all the water in one go
%         \task Pour in a slow, steady spiral from center to edge
%         \task Pour only in the center
%         \task Pour randomly across the coffee bed
%     \end{tasks}

%     \item How should we decide when to add water during brewing?
%     \begin{tasks}(1)
%         \task Pour all the water at once at the beginning
%         \task Add water whenever the coffee bed becomes visible
%         \task Add water only when the previous pour has fully drained
%         \task Pour water based on the color of the coffee dripping out
%         \task Add water whenever the brewing slows down significantly
%     \end{tasks}

%     \item Should you use a higher water temperature for a darker roast of coffee beans?
%     \begin{tasks}(1)
%         \task Yes, darker roasts need higher temperatures
%         \task No, use a lower temperature for darker roasts
%         \task The temperature should be the same for all roasts
%         \task Alternate between high and low temperatures
%     \end{tasks}

%     \item Which combination of factors is most likely to result in over-extraction (i.e., coffee tastes too bitter)?
%     \begin{tasks}(1)
%         \task Fine grind, low temperature, fast pour
%         \task Coarse grind, high temperature, slow pour
%         \task Fine grind, high temperature, long brew time
%         \task Coarse grind, low temperature, short brew time
%     \end{tasks}

%     \item Why should we pour the water multiple times instead of all at once?
%     \begin{tasks}(1)
%         \task For temperature consistency and even extraction
%         \task To make the coffee more sour
%         \task To extend the brewing time, making the coffee stronger
%         \task To allow the coffee grounds to absorb more air, enhancing the coffee's aroma
%     \end{tasks} 
% \end{enumerate}

%  Below is the quiz for Task B.
% \begin{enumerate}[label=\textbf{Q\arabic*.}]
%     \item Which part of the breadboard is typically used as the power rail?
%     \begin{tasks}(2)
%         \task The long strips on the sides
%         \task The lettered columns
%         \task The numbered rows
%         \task The center divide
%     \end{tasks} 

%     \item In this circuit, what is the purpose of the resistors?
%     \begin{tasks}(2)
%         \task To increase the voltage
%         \task To store energy
%         \task To limit current to the LEDs
%         \task To increase the brightness of LEDs
%     \end{tasks}

%     \item What would happen if you reversed the battery connections in your circuit?
%     \begin{tasks}(2)
%         \task The LEDs would light up brighter
%         \task The circuit would short circuit
%         \task The resistors would burn out
%         \task The LEDs would not light up
%     \end{tasks}

%     \item If one LED fails in your circuit, what happens to the others?
%     \begin{tasks}(2)
%         \task They all go out
%         \task They remain lit
%         \task They flicker
%         \task They become brighter
%     \end{tasks}

%     \item What would be the effect of adding more LEDs in parallel to this circuit?
%     \begin{tasks}(2)
%         \task The LEDs would become brighter
%         \task The circuit would stop working
%         \task The resistors would \\overheat
%         \task The power would drain faster
%     \end{tasks}

%     \item Which connection below is wrong if you want to connect the resistor in a circuit? (See Fig. \ref{fig:breadboard})
%     \begin{tasks}(3)
%         \task A
%         \task B
%         \task C
%         \task D
%         \task None of the above
%     \end{tasks}
    
%     \begin{figure}
%         \centering
%         \includegraphics[width=0.5\linewidth]{figures/breadboard.png}
%         \caption{Question 6 figure.}
%         \label{fig:breadboard}
%     \end{figure}

%     \item Will both red LEDs light up? (See Fig \ref{fig:redled}
%     \begin{tasks}
%         \task Yes
%         \task No
%         \task Not sure
%     \end{tasks}

%     \item Would it make a difference if we removed one of the resistors? (See Fig \ref{fig:redled}
%     \begin{tasks}
%         \task Yes
%         \task No
%         \task Not sure
%     \end{tasks}

% \begin{figure}[h]
%     \centering
%     \subfloat[Figure for Questions 7 and 8.]{
%         \includegraphics[width=0.25\textwidth]{figures/redled.png}
%         \label{fig:redled}
%     }
%     % \hspace{1em}  % Add space between subfloats
%     \subfloat[Figure for Question 9.]{
%         \includegraphics[width=0.25\textwidth]{figures/blueled.png}
%         \label{fig:blueled}
%     }
%     \caption{LED configurations}
%     \label{fig:leds}
% \end{figure}

%     \item The voltage required for a red LED to light up is 1.8V, while that for a blue LED is 3V. Will both LED light up here?  (See Fig \ref{fig:blueled}
%     \begin{tasks}
%         \task Yes
%         \task No
%         \task Not sure
%     \end{tasks}

%     \item In the circuit you assembled, would all LEDs still light up if you replaced 2 of them with blue LEDs?
%     \begin{tasks}
%         \task Yes
%         \task No
%         \task Not sure
%     \end{tasks}

%     \item What is the benefit of using a breadboard? (Select all that apply)
%     \begin{tasks}
%         \task Components can be added and removed easily
%         \task Holes are internally connected so that we don't have to solder
%         \task It can be reused and modified easily
%     \end{tasks}
% \end{enumerate}
